# Supplementary material for: State space modelling and data analysis exercises in LISA Pathfinder
Source: arXiv:1306.4487 source file (2013-06-21)
Supplement: Supplementary file 1 [file appendix.tex]

\appendix

\section{balh}
